# Supplementary material for: A systematic review of relation extraction task since the emergence of Transformers
Source: arXiv:2511.03610 source file (2025-11-21)
Supplement: Supplementary file 1 [file 0_supplMat.tex]

\section{Introduction}
The increasing digitalisation of daily life has led to the creation of vast volumes of textual data that organisations and individuals must manage. Within these extensive digital repositories, the task of relation extraction (RE) plays a crucial role. RE refers to the process of structuring knowledge from unstructured textual content, thereby enabling more effective indexing, description, search, and retrieval of specific information from large-scale corpora. The demand for relation extraction has grown significantly due to the exponential increase in machine-readable text, particularly since the advent of the World Wide Web in 1989~\cite{bernerslee1989information}. This explosion of information also motivated Tim Berners-Lee to propose the concept of the Semantic Web~\cite{bernerslee2001semantic}, a vision aimed at enabling machines to understand and reason over web content. A core instantiation of Semantic Web principles is the knowledge graph (KG), in which nodes represent entities of interest and edges denote the semantic relations between them. Initially popularised by Google through the creation of the Google Knowledge Graph, KGs are now widely employed across industry and academia for tasks involving structured reasoning and information retrieval. To support such applications, several large-scale, openly available knowledge bases have been developed, including Freebase~\cite{10.1145/1376616.1376746}, YAGO~\cite{10.1145/1242572.1242667}, DBpedia~\cite{10.1007/978-3-540-76298-0_52}, and Wikidata~\cite{10.1145/2629489}. These resources are the result of collaborative, community-driven efforts to collect and maintain millions of factual assertions. However, ensuring both the quality and completeness of these knowledge bases remains a challenging and labour-intensive task. In this context, relation extraction serves as a vital mechanism for automatically enriching and correcting knowledge graphs using evidence drawn from textual corpora. While KGs may be viewed as the end product, RE represents the foundational process by which new structured knowledge is identified and integrated from unstructured sources.

The research field of \textbf{relation extraction} (RE) and knowledge acquisition from text spans more than three decades. A key milestone in its early development was the \textit{Fourth Message Understanding Conference} (MUC-4) in 1992, which introduced the first standardized evaluation metrics---\textit{precision} and \textit{recall}---and presented the first RE system, \textit{Fastus}~\cite{hobbs-etal-1993-fastus} (Finite State Automaton Text Understanding System), thereby paving the way for rule-based systems. Since these foundations, RE has undergone significant evolution, propelled by advances in machine learning---initially through statistical approaches and, more recently, through deep learning techniques---marking a decisive shift towards neural architectures. In particular, the emergence of large-scale pre-trained language models~\cite{devlin-etal-2019-bert,NEURIPS2020_1457c0d6} based on transformer architectures has led to substantial performance gains across a wide spectrum of canonical natural language processing (NLP) tasks~\cite{wang-etal-2018-glue}. These developments have reinvigorated research interest in RE, particularly within the \textbf{knowledge management} and \textbf{information extraction} communities~\cite{DBLP:conf/emnlp/PetroniRRLBWM19,razniewski2021languagemodelsknowledgebases,pan_et_al:TGDK.1.1.2,zheng2024reliablellmsknowledgebases}, and have driven a notable increase in research activity.

\paragraph{Previous Surveys.} 
As detailed in Section~[SEC], numerous surveys on RE are published each year. However, only a small subset follow a rigorous systematic review methodology. Our collection process identified six systematic reviews published since 2020. The first of these, by~\cite{martinez-rodriguez_information_2020}, has become a key reference for researchers addressing semantic relation extraction, as it comprehensively covers all subtasks of RE and provides an extensive overview of pre-2020 resources and tools. While still valuable, its coverage is limited to models based primarily on pipeline architectures and rule-based methods, which are now outdated. Last notable works include~\cite{nasar_named_2021}, which addresses grammar checking and incorporates RE as a subtask in that context, and~\cite{yohan_bonescki_gumiel_temporal_2021}, which focuses on event relation extraction. The 2022 survey by~\cite{bassignana_what_2022} centers on dataset creation and the impact of annotation choices on model performance. More recent studies, such as~\cite{schneider_decade_2022} and~\cite{lingfeng_zhong_comprehensive_2023}, provide higher-level perspectives on knowledge graph construction but devote comparatively less attention to the specific challenges of RE.

\paragraph{Positioning.} 
This systematic review is designed to capture and analyze research developments in RE \textbf{since the advent of Transformer architectures}, with a dual focus on available \textbf{resources} and the \textbf{models} developed to address the task. By applying a rigorous and extended systematic process, we offer an updated and detailed state-of-the-art overview. All data generated during this study is openly released, enabling reuse and supporting future investigations.

\paragraph{Objectives of this Review.} 
The aim of this work is to deliver a comprehensive synthesis of current RE research through an \textbf{extended systematic literature review (SLR)}, focusing on the period \textbf{2019--2024} following the introduction of Transformer-based models~\cite{10.5555/3295222.3295349}.

Our review addresses three key aspects: 
\begin{enumerate}
   \item \textbf{Survey literature} on RE;
   \item \textbf{Models} proposed to solve the RE task;
   \item \textbf{Datasets} used for model training and evaluation.
\end{enumerate}

Through iterative filtering, categorization, and annotation, we analyze more than \textbf{30 dimensions} of the research landscape to address the following research questions:
\begin{itemize}
   \item \textbf{RQ1:} What resources have been developed to address the RE task, and how are they integrated with knowledge bases (KBs)?
   \item \textbf{RQ2:} Which models have been proposed since the introduction of Transformer architectures?
   \item \textbf{RQ3:} How have researchers combined resources and models to solve and formalize the RE task?
\end{itemize}

Our contributions are as follows:
\begin{enumerate}
   \item We present an updated overview of RE research, emphasizing the transformative impact of large language models.
   \item We apply a novel extended SLR framework (\textbf{SciLex}) that enables the systematic collection and enrichment of scientific publications for state-of-the-art studies.
   \item We provide a fine-grained, consistent, and detailed data extraction---unprecedented in RE surveys---which is made openly accessible to the community.
\end{enumerate}

The SciLex toolbox also allows us in this context to point the missing dimension to annotate.  Previous work related to NLP tasks already underlines the importance of pre-annotation steps [Fort and Sagot, 2010] and annotation tools [Dandapat et al., 2009] to avoid annotation bias as well as annotation guidelines [Nedelec.]. 

To getting back to the relation extraction task (RE) covers and consists of several steps: first, identifying entities (ex, person, company name, a specific molecule), keywords, or a span of text (argument, events), as well as a date. An entity typing step (ET) could extend the detection of the entities covered. In the second step, the entity discovered could be linked to a knowledge base by retrieving the unique identifier used to refer to it, this step is also known as under the name of entity linking (EL). The final step generally relates to identifying (or classification) relations between concepts covered in a text, which is also called the relation classification (RC) step. This task could be addressed at different granularities, from sentences to entirely unstructured documents. The coreference detection (noted Coref) step could be leveraged in second cases.  The recent development of effective language models trained on large corpora of mixed web content demonstrated an impressive performance gain in many Information-intensive tasks and consequently engaged much research in this direction.

It serve as base of a large number of use case as search engines, question answering, and could be applied to many application domain. DO RESEARCH ABOUT APPLICATIONS

SOURCE OF INSPIRATION FOR INTRO : 
https://arxiv.org/pdf/2308.06374
https://arxiv.org/pdf/2501.06699
https://arxiv.org/abs/2411.04920
https://arxiv.org/abs/2204.06031
http://arxiv.org/abs/1909.01066
http://arxiv.org/abs/2110.04888

These documents could take many forms, from unstructured text to structured ones (e.g., web pages), tables, or even images or videos. 
This systematic review of the literature focuses on a specific kind of information extraction, which is called relation extraction. The research question of relation extraction and knowledge acquisition from text has a history of over 30 years. If we consider a first and concrete milestone, the 4th Message Understanding Conference of 1992 introduced the initial evaluation metrics (precision, recall). It proposed the first model for relation extraction called Fastus (Finite State Automaton Text Understanding System). However, rule-based systems like Fastus quickly encountered issues related to combinatorial complexity and semantic ambiguity.

During the last decade, researchers designed more complex models based on features and multistep pipelines that were finally based on both worlds (natural language processing and knowledge graphs): named entity recognition, entity linking, relation extraction, and relation classification. Further progress was also made in defining annotation standards, creating multidisciplinary corpora and establishing metrics. Nevertheless, this design often leads to the accumulation of errors throughout the subtasks, which directly impacts the overall performance of the models.

\subsection{An extended Systematic literature Reviews}
Science publication is significantly growing as well as the access to it thought open initiatives~\cite{hanson2024strainscientificpublishing}. In the first instance, this is for researchers the opportunity to enter the state-of-art realm; unfortunately, the other side of the coin is now to filter these potentially massive corpora only to only to a given research question by meeting certain quality criteria. 
Moreover, science is today face to a crisis of reproducibility~\cite{COHENBOULAKIA2017284}, which must be taken into account by researchers to leverage existing literature. In fact, bias / shortcoming could easily be impacted by a lack of transparency~\cite{Haibe-Kains2020}.  
Systematic literature reviews (SLR) is a rigorous solution, requiring  a well-defined methodology, allowing to assess and compare previous research done on a given topic. Nevertheless SLR require considerably more effort than traditional surveys or reviews~\cite{kitchenham_guidelines_2007}.  

In the first hand, many tools and software are today available proposing to help the analysis of a literature corpora notably by integrating machine learning~\cite{bolanos2024artificialintelligenceliteraturereviews} but their are generally limited to a given purpose.    
On the other hand, a lot a services are today available making articles: 1. referenciable (DOI) 2. interlinkable (CROSSREF) 3. evaluable on the point of view of the performances (PaperWithCode\cite{stojnic_papers_2019},\cite{kardas_axcell_2020}). 

This article is in this direction proposing a framework: SciLEx, made to explore, expand, analyse and annotate a scientific corpora.   

PapersWithCode is a platform  that "help the community to track newly published machine learning papers with source code and quickly understand the current state of the art". Created in 2018, this one is today hosted by MetaIA under a CC-BY-SA license . Firstly based on aggregation on hand-annotated benchmark (NLP-progress, EFF, RedditSota, SQuAD, SNLI), the website also allows crowdsourcing : by leaving the possibility to add new papers, new tasks, gives the option to enter manually performances metrics of the models benchmarked. However, as publications on machine learning are very numerous and tend to increase continuously, they created a partnership with Arxiv in 2020 in order to speed up the coverage of the plateform. This one offers to authors the opportunity to links machine learning papers to the official gihtub repository \cite{stojnic_papers_2020} containing the code used for the experiments. The PapersWithCode team also proposed a solution for facilitating the extraction of the experimental results from papers \cite{kardas_axcell_2020}, by this way they are able to detect dataset mentions, cited models, task solved and metrics.

\subsection{The Relation extraction task}

The digitalization of every aspect of today's life has given access to a plethora of documents that every actor has to manage: from the industry to institutions, as well as scientists. In these giant digital libraries of text, the relation extraction task consists of "structuring knowledge from unstructured texts", which is helpful to better index, describe, search, and retrieve specific pieces of information.      

This makes the research fields actuaThis is generally done by identifying significant facts that link objects, concepts, and measures from a given textual corpus. 

Relation extraction needs has arisen due to the exponential growth in computationally processable text, notably since the inception of the web in 1989[citation]. The research question of relation extraction and knowledge acquisition has a history of over 30 years. If we consider as a first and concrete milestone the 4th Message Understanding Conference of 1992 that introduced the initial evaluation metrics (precision, recall) and proposed the first model for relation extraction called Fastus (Finite State Automaton Text Understanding System). However, rule-based systems like Fastus quickly encountered issues related to combinatorial complexity and semantic ambiguity.

The Semantic Web, designed as a semantic extension of the web by Timm Bernes Lee, has been standardized and promoted by the W3C since 1994. The consortium addressed the issue of sharing knowledge and information via the web while developing concepts and tools for identifying and sharing data (using URI), representing data (using RDF format), building ontologies (using OWL), querying structured data on the web (using SPARQL), and reasoning on it (using RIF). These initiatives fostered the creation of Linked Open Data, which comprises knowledge bases that adhere to Semantic Web principles. The most renowned examples of which are knowledge bases are DBpedia and Wikidata both built for describing Wikipedia entities. The first one is multilingual and based on the development of extractors that leverage infoboxes information, the second is the result of a crowdsourcing and robots assistance initiative that centralize all possible chapters entities. These knowledge bases are not based on the information of the Wikipedia articles, but offers the possibility to align text and graphs of relations derived from their. 

Researchers designed more complex models based on features and multistep pipelines that were finally based on both worlds (natural language processing and knowledge graphs): named entity recognition, entity linking, relation extraction, and relation classification. Further progress was also made in defining annotation standards, creating multidisciplinary corpora and establishing metrics. Nevertheless, this design often leads to the accumulation of errors throughout the subtasks, which directly impacts the overall performance of the models.

Recently, natural language processing techniques have witnessed significant improvements through advancements in deep learning: from word2vec to sequential multi-layer perceptron and transformer architectures. They are based on a first learning phase that tries to forecast previous and next words in a given sequence of words. These systems allowed us to encode larger context and integrate complex patterns from natural language, by learning on massive web corpora. 

Last generation of transformer based models expanded not only in size but also in terms of transferability. The recent commercial demonstration has shown the capacity of generative tasks to be good in natural language understanding in a wide range of contexts.

This survey captures today's landscape drawn around the relation extraction task, a research dynamic research field in the intersection of NLP and Knowledge graph domain. The study is the result of a systematic literature review made on this period and conducted thanks to an original methodology. We present our kick-started process tertiary study in part II. of this paper, from the first large Digital Libraries API exploitation of the surveys published since 2010 and today. We consolidate these results via PapersWithCode, CrossRef, and Open Citation sources which led us to build a vast network of works we interrogate via a well-defined selection protocol. We present this in part III. data resulting from this first collection, and we also present the quality and the annotation protocol we choose to follow. Part IV. of this paper deserves the analysis of the corpora we built regarding our research question.

\subsection{Research Questions approached }

In this survey we would to answer the following research questions related to a Relation Extraction task:
How to learn efficient customized extractors targeting specific RDF patterns from the dual base formed by a corpora of text on one hand, and Knowledge bases on the other hand?

So the initial purposes of this systematic review are the five following subresearch questions:
\begin{itemize}
   \item SRQ.1 – How the recent literature is modeling this problem by using Deep learning architectures and Languages models to solve it ?   
   \item SRQ.2 – How the chose made in the design of the input/output impact the task ? 
   \item SRQ.3 – To what extent the training data and process impact the relation extraction task ? 
    \item SRQ.4 – How the current state of the art is dealing with under-represented fact ? 
\end{itemize}
The SciLEX collects, will also allow us to measure also others quality 
Which dataset was built to solve the task ? 
How do the model perform on benchmark ? And which are the current challenges ?
What is the dynamic of the publication process around our question?

\begin{table}[ht]
\centering
\begin{tabular}{p{4cm}|p{5cm}|p{5cm}}
\hline
\textbf{Feature} & \textbf{Closed Relation Extraction} & \textbf{Open Relation Extraction} \\
\hline
Relation schema & Predefined, fixed set & Unbounded, extracted from text \\
\hline
Relation label & Formal ontology or predicate & Free-text phrase (e.g., verb) \\
\hline
Supervision & Supervised (requires labeled training data) & Unsupervised or weakly supervised \\
\hline
Integration with KG & Straightforward (mapped to existing schema) & More challenging (requires canonicalization/mapping) \\
\hline
Example output & \texttt{(Marie Curie, dbo:birthPlace, Warsaw)} & \texttt{(Marie Curie, "was born in", Warsaw)} \\
\hline
Use cases & KG population, question answering, entity linking & Web-scale mining, bootstrapping knowledge bases \\
\end{tabular}
\caption{Comparison of Closed vs Open Relation Extraction}
\label{tab:closed-vs-open-re}
\end{table}

\subsubsection{Knowledge Graphs}
A knowledge graph (KG) can be formally defined as a directed labelled graph:
\[
\mathcal{G} = (E, R, T)
\]
where:
\begin{itemize}
    \item $E$ is a finite set of \textit{entities} (nodes or vertices),
    \item $R$ is a finite set of \textit{relations} (edge types or predicates),
    \item $T \subseteq E \times R \times (E \cup L)$ is a set of \textit{triples} or \textit{facts}.
\end{itemize}
Each triple is of the form $(s, p, o)$, where $s \in E$ is the \textbf{subject entity}, $p \in R$ is a \textbf{relation} (also known as a \textit{property}), and $o \in E \cup L$ is the \textbf{object}, which can be either another entity or a literal.

\subsubsection{Entities}~\label{def:entities}
Entities represent real-world objects or abstract concepts and form the fundamental units of a knowledge graph. Examples include people, locations, organisations, events, or ideas. When an entity can be uniquely identified, it is typically referred to as a \textit{named entity}. Entities may also be associated with types, as explained in the section on classes. Detecting entities from text generally relates to Named Entity Recognition~\ref{def:ner}.

\subsubsection{Labels}~\label{def:label}
A label is a human-readable string that serves as the descriptive name of an entity—e.g., “Paris”. Unlike identifiers, labels are not unique and may refer to multiple entities. Trying to extract from text, labels related to entities and corresponds to Mention Detection~\ref{def:mention_detect}.

\subsubsection{Identifiers}~\label{def:identifier}
Each entity $e \in E$ is associated with a unique identifier to ensure unambiguous reference:
\[
id: E \rightarrow \mathcal{I}
\]
Identifiers are often represented as IRIs (Internationalised Resource Identifiers)—an extension of URIs (Uniform Resource Identifiers) that supports Unicode. For instance, in Wikidata, the city of Paris is identified as:
\[
id(\text{Paris}) = \texttt{Q90} \quad \text{(Wikidata URI: \url{https://www.wikidata.org/entity/Q90})}
\]
In DBpedia, the same entity is referred to as:
\[
id(\text{Paris}) = \texttt{http://dbpedia.org/resource/Paris}
\]
Being able to attach a unique identifier relates to the Entity Linking task~\ref{def:EL}. 

\subsubsection{Relations}~\label{def:relations}
Relations (also called properties or predicates) link entities to other entities or to literal values. They are typically directed. When a relation connects two entities, it is known as an \textit{object property}. Conversely, if the relation connects an entity to a literal value (such as a date, string, or number), it is referred to as a \textit{datatype property}. Being able to identify which relations are expressed by two entities in a text segment is generally part of the Relation Identification task~\ref{def:RI}, when identifying the relations with a unique ID could be considered as the relation classification task~\ref{def:RC}.

\subsubsection{Triples}~\label{def:triple}
A triple is the atomic unit of information in a KG, encoding a single fact. It comprises a subject entity, a relation, and an object, which may be either an entity or a literal. This can be formalised as:
\[
T \subseteq E \times R \times (E \cup L)
\]
where $L$ denotes the set of literals.
Extracting triples from text is the special focus of our surveys and is generally referred as the Relation extraction task~\ref{def:RE}.

\subsubsection{Classes}~\label{def:class}
Entities in a KG are often described according to a classification system based on shared characteristics. These \textit{classes} are typically structured hierarchically via \textit{subclass} relationships. Algebraically, we denote the set of classes as $C \subseteq E$, and the class membership of an entity $e \in E$ is expressed via a triple:
\[
(e, \texttt{type}, C)
\]
For example, the entity \texttt{Victor\_Hugo} being of type \texttt{Person} would be recorded as: \texttt{(Victor\_Hugo, type, Person)}. Class hierarchies support logical inference and schema validation in the KG. Attaching a type to an entity could be included in the NER task~\ref{def:ner}, and is especially refered as the Entity Typing task~\ref{def:ET}

\subsubsection{Ontology}~\label{def:ontology}
An ontology defines the conceptual schema of a knowledge graph. It specifies:
\begin{itemize}
    \item The set of allowed \textbf{classes} ($C$),
    \item The set of defined \textbf{relations} or \textbf{properties} ($R$),
    \item A set of \textbf{axioms or constraints} ($A$).
\end{itemize}
Formally, we write:
\[
\mathcal{O} = (C, R, A)
\]
Common axiom types include:
\begin{itemize}
    \item \textit{Subclass hierarchies}: $c_1 \sqsubseteq c_2$, denoting that $c_1$ is a subclass of $c_2$.
    \item \textit{Relation constraints}: domain and range restrictions. Given a triple $(e_1, r, e_2)$, the \textbf{domain} of $r$ specifies the class of $e_1$ (the subject), and the \textbf{range} specifies the class of $e_2$ (the object).
\end{itemize}

\subsubsection{TBox and ABox}~\label{def:tbox_abox}
Knowledge graphs are typically understood as the combination of two components:
\begin{itemize}
    \item The \textbf{TBox} (Terminological Box), which contains the ontology—i.e., the schema, classes, and axioms.
    \item The \textbf{ABox} (Assertional Box), which contains instance-level data—i.e., the actual entity-relation-entity or entity-relation-literal assertions.
\end{itemize}
Together, these components provide both the conceptual structure and the factual content of a knowledge graph. Both levels could be discovering or inferred by text by design it as a relation extraction task.

\subsection{Semantic Web Standards}

The World Wide Web Consortium (W3C) is responsible for developing open, interoperable standards to ensure the long-term growth and accessibility of the Web. In addition to widely adopted standards for document structure and presentation—such as HTML, CSS, and XML—the W3C has also defined a suite of specifications supporting the Semantic Web and Linked Data. These include URI, RDF, OWL, SHACL, and SPARQL.

\begin{itemize}
    \item \textbf{URI (Uniform Resource Identifier):}~\label{def:uri}\footnote{\url{https://www.w3.org/Addressing/URL/uri-spec.html}} As discussed in the previous section, URIs provide a globally unique means of identifying web resources. They enable dereferencing, allowing users and systems to retrieve representations of identified resources via standard web protocols.
    
    \item \textbf{RDF (Resource Description Framework):}~\label{def:rdf}\footnote{\url{https://www.w3.org/TR/rdf-schema/}} RDF is a standard model for representing structured information on the Web. It encodes knowledge as a set of triples—\textit{subject}, \textit{predicate}, and \textit{object}—forming a graph-based data model. RDF supports the integration of structured and semi-structured data from diverse sources by using URIs and literals as its atomic elements. RDF-star~\footnote{\url{https://w3c.github.io/rdf-star/cg-spec/editors_draft.html}} actually in discussion, extends RDF to express easily n-ary relations.  
    
    \item \textbf{OWL (Web Ontology Language):}~\label{def:owl}\footnote{\url{https://www.w3.org/TR/owl-features/}} OWL is a language designed for defining and instantiating ontologies on the Web. Built atop RDF, it allows the specification of classes, properties, and logical axioms. OWL enables automated reasoning, supporting inference over class hierarchies, property constraints, and entity relationships.
    
    \item \textbf{SHACL (Shapes Constraint Language):}\footnote{\url{https://www.w3.org/TR/shacl/}} SHACL is a standard language for validating RDF graphs against a set of conditions or constraints. It defines “shapes” that describe expected graph structures and value ranges, supporting data quality control and consistency enforcement.
    
    \item \textbf{SPARQL (SPARQL Protocol and RDF Query Language):}~\label{def:sparql}\footnote{\url{https://www.w3.org/TR/sparql11-query/}} SPARQL is the standard query language for RDF datasets. Functionally analogous to SQL for relational databases, SPARQL supports pattern matching on graph data and includes a variety of query operators tailored for navigating and retrieving information from RDF graphs.
\end{itemize}

\begin{center}
\begin{figure}[h!]
\begin{minipage}[c]{\textwidth}
\centering
    \includegraphics[width=3.0in]{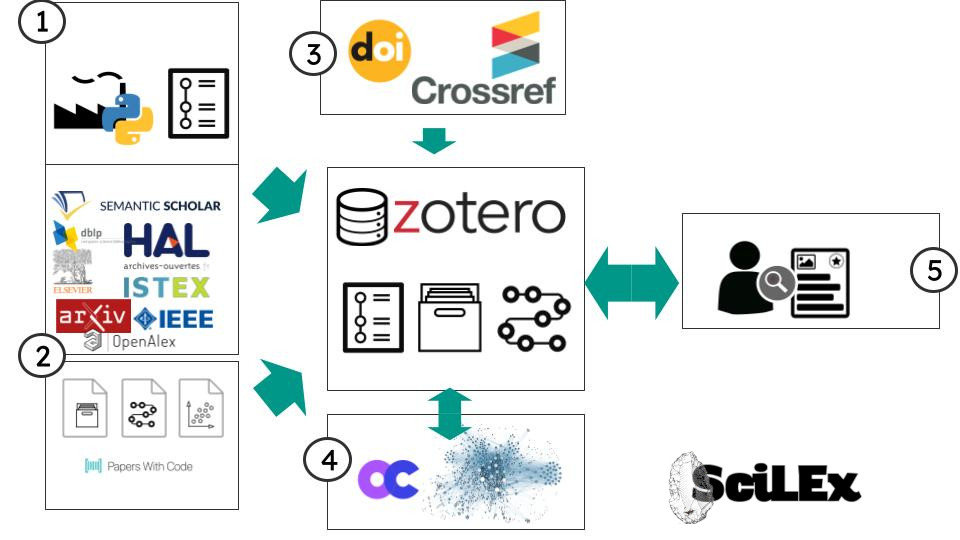}
    \caption{overview SciLEX framework}
    \label{fig:scilex_framework}
\end{minipage}
\end{figure}
\end{center}
\begin{figure}[h!]
\begin{minipage}[c]{\textwidth}
\centering
    \includegraphics[width=.6\linewidth]{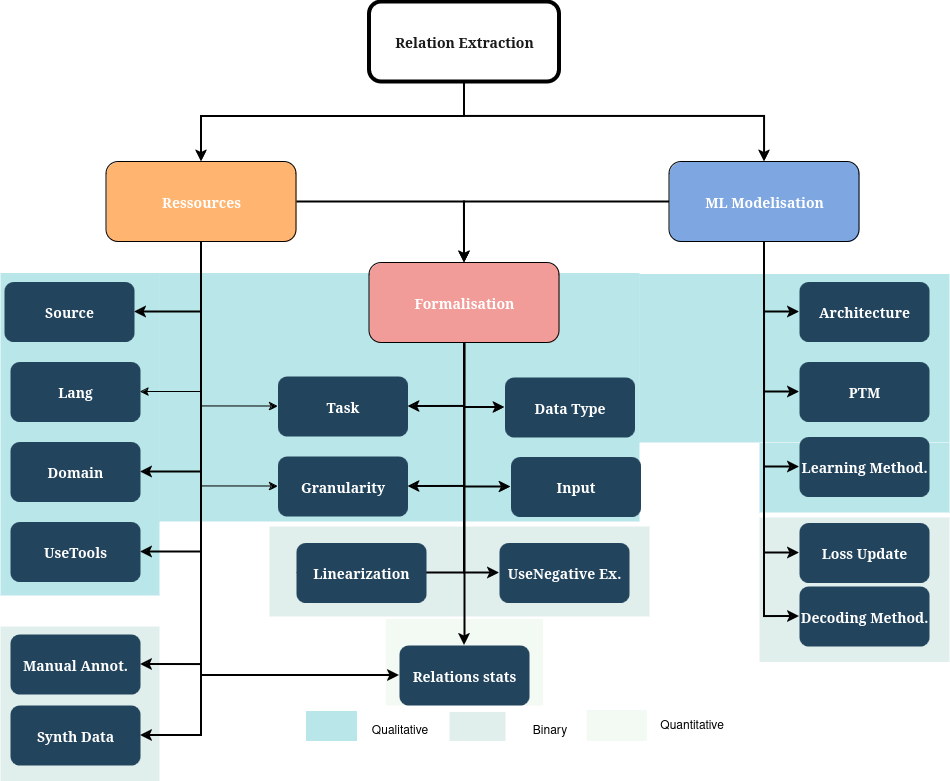}
    \caption{Analyse dimensions overview}
    \label{fig:sample_figure}
\end{minipage}
\end{figure}

\subsection{Open Challenges }

\subsection{Semantic Web Integration and Knowledge Graph Alignment}

While some surveys and datasets incorporate Semantic Web resources (e.g., DBpedia, Wikidata)
, their potential remains underexploited. Explicit alignment between RE outputs and structured ontologies can support better reasoning and interoperability. Future directions include:

Joint learning approaches that align RE tasks with ontology constraints (e.g., domain and range axioms).

Integration with KG completion and reasoning tasks to create unified knowledge acquisition pipelines.

Development of benchmarks where RE outputs are evaluated not only on textual accuracy but also on their utility for downstream KG applications.

\subsection{Evaluation Practices and Reproducibility}

Our meta-analysis of benchmarking practices revealed inconsistencies in evaluation settings, dataset splits, and reported metrics across studies. In addition, while some models provide open code and trained checkpoints, many do not
. To improve reproducibility and comparability:

Standardized evaluation suites (e.g., KILT [81]) should be extended and adopted more widely.

Transparent reporting guidelines, including dataset splits, hyperparameters, and negative examples, should be followed.

Long-term sustainability of resources is essential; links to code, datasets, and pretrained models should remain persistent.

\subsection{Generative and Knowledge-Intensive RE}

The recent trend towards generative RE (e.g., REBEL [44], WDV [10]) opens new research avenues but raises challenges in factuality and controllability. Future work should explore:

Controllable text-to-triple generation using constrained decoding aligned with KG schemas.

Hallucination mitigation strategies, ensuring generated relations correspond to verifiable facts.

Unified evaluation benchmarks that compare generative and extractive approaches under the same protocols.

Summary of Future Directions: To address these challenges, we recommend a combined focus on high-quality multilingual resources, cross-document reasoning, Semantic Web integration, and standardized evaluation practices. As RE becomes increasingly central to knowledge acquisition pipelines, collaboration between the NLP and Semantic Web communities—as initiated in works like Martinez-Rodriguez et al. [68] and expanded here—will be crucial to push the boundaries of scalable and reliable information extraction.

\section{Conclusion}

A complete shift from classification to generative models
The usage of SLM to
